# Supplementary material for: Multi-modal Causal Structure Learning and Root Cause Analysis
Source: arXiv:2402.02357 source file (2024-02-04)
Supplement: Supplementary file 1 [file Appendix.tex]

\section{Extracting Label Information for Log Representation Learning}
\label{log_representation_appendix}
The extracting label information process involves partitioning the collected system logs into fixed time windows. For each of these windows, we create a log sequence, capturing unique log templates occurring within that specific time frame. In typical large language models, individual words in a sentence are treated as tokens. However, this approach isn't suitable for log sequence representation learning for two main reasons.

Firstly, the presence of a significant number of infrequent special tokens makes it challenging to learn effective representations for these tokens, given the limited sample size. Secondly, tokenizing log templates into lists of word tokens requires setting a very large maximal sequence length to accommodate all sequences within that limit. However, this can be problematic since, in practice, time windows are often set to $10$ to $30$ minutes to gather more valuable and reliable information. In some cases, the number of unique log templates exceeds $50$, and when each word in these log templates is tokenized, the sequence length of the log sequence surpasses the default maximal sequence length (\eg, $512$) used in traditional large language models. When the sequence length exceeds this limit, the exceeding part is truncated, leading to information loss. 

Conversely, having an extensive maximal sequence length poses multiple challenges. Firstly, it demands a substantial GPU memory and prolongs the training time, making it less feasible for practical deployment. This becomes particularly problematic when implementing an online system, which typically operates under tight time constraints. Online systems need to produce results before the arrival of the next batch of new data. Therefore, a large maximal sequence length becomes a hindrance to the deployment of online systems. Moreover, obtaining precise label information for log event templates presents a substantial challenge. The labeling process can be costly, and it often necessitates expert knowledge. The absence of high-quality label information poses a significant impediment to the ability of large language models to effectively learn the desired high-quality representations.

To address these challenges, our approach begins by capturing all unique log event templates within the specified time windows. We then transform the log sequence into a sequence of event template tokens using a specialized tokenizer. In this unique approach, each event template is treated as an individual token, as illustrated in Figure~\ref{fig:mulan_log_representation}. In addition, different from the traditional large language, we also consider the frequency of each unique log template as the more frequently a log event template appears, the more important message it carries. This assumption proves highly valuable in addressing certain failure scenarios, such as Distributed Denial of Service (DDoS) attacks. During a DDoS attack, certain log event templates may experience a sudden, significant increase in frequency, signaling unusual behavior. Thus, we include the frequency information alongside each log event template, providing extra context to detect unusual patterns in potential failure cases.

%To address these challenges, we first record all unique log event templates in the given time windows and transform the log sequence into a sequence of event template tokens using a tokenizer by considering each event template as a token shown in Figure~\ref{fig:mulan_log_representation}. In addition, different from the traditional large language, we also consider the frequency of each unique log template as the more frequently a log event template appears, the more important message it carries. This assumption may be extremely useful to deal with some failure cases, such as DDoS attacks. When a DDoS attack occurs, the frequency of some log event templates will suddenly increase dramatically, indicating unusual behaviors. By adding the frequency right after each log event template, we incorporate the extra information to monitor these usual patterns for some potential failure cases. 

To address the challenge of lacking label information, we propose two viable solutions. The first method is a "golden signal" approach that leverages domain knowledge. For instance, consider a microservice system, where system failures can be classified into various types, including DDoS attacks, storage failures, high CPU utilization, high memory utilization, and more. Each type of system failure is associated with specific keywords or "golden signals." By identifying these keywords within log event templates, we can determine whether a particular template is abnormal. These keywords may include terms like "error," "exception," "critical," "fatal," "timeout," "connection refused," "No space left on the device," "out of memory," "terminated unexpectedly," "backtrace," "stack trace," "service unavailable," "502 Bad Gateway," "503 Service Unavailable," "504 Gateway Timeout," "unable to connect to," "rate limit exceeded," "request limit exceeded," "cloud system down," "cloud service not responding," "failure," "corrupted data," "data loss," "file not found," "high CPU utilization," "CPU spike," "CPU saturation," "excessive CPU usage," "failed," "shutdown," "Permission denied," "DEBUG," and more. The presence and extent of these abnormal log event templates within a log sequence are measured to compute the overall abnormality of the sequence, which serves as label information. When domain knowledge is not readily available, our second solution involves using anomaly detection models, such as Deeplog~\cite{DBLP:conf/ccs/Du0ZS17} or OC4Seq~\cite{DBLP:conf/kdd/WangCNLCT21}, to evaluate the abnormality of a log sequence.

\section{Additional Experiment}

\begin{figure*}
\begin{center}
\begin{tabular}{ccccc}
\hspace{-5mm}
\includegraphics[width=0.18\linewidth]{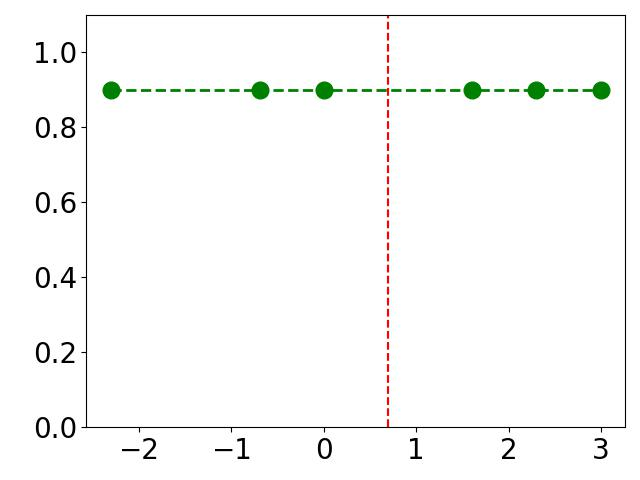} &
\includegraphics[width=0.18\linewidth]{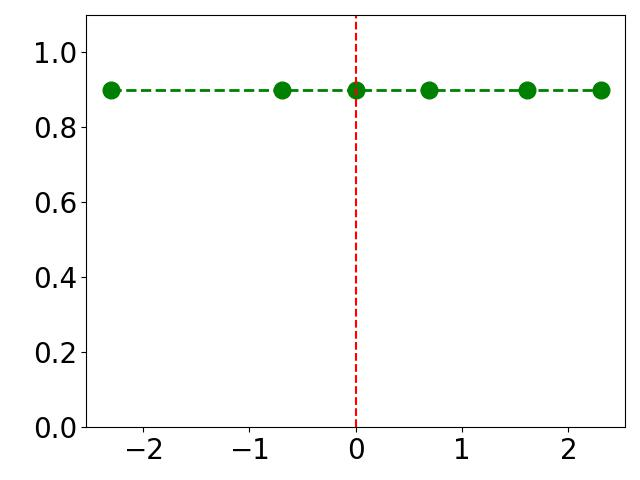} &
\includegraphics[width=0.18\linewidth]{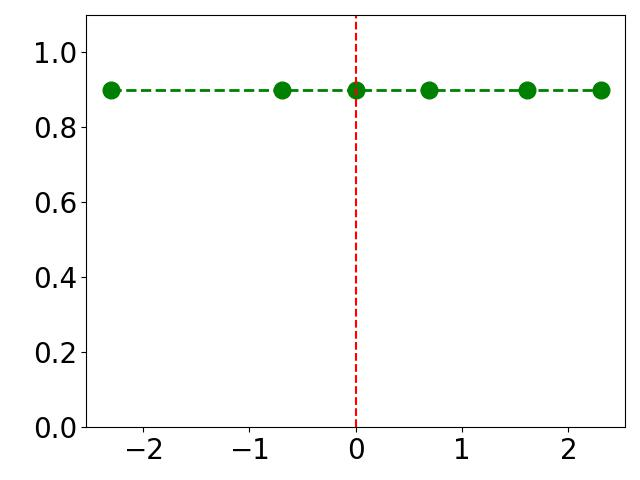} &
\includegraphics[width=0.18\linewidth]{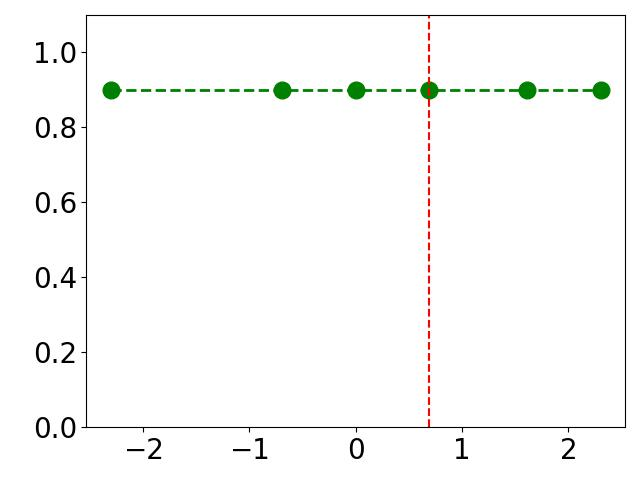} &
\includegraphics[width=0.18\linewidth]{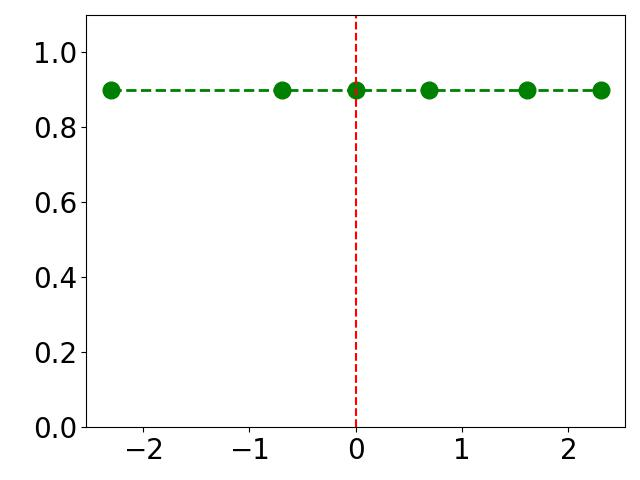}\\
(a) $\log(\lambda_1)$ {\it w.r.t.} MRR&
(b) $\log(\lambda_2)$ {\it w.r.t.} MRR &
(c) $\log(\lambda_3)$ {\it w.r.t.} MRR &
(d) $\log(\lambda_4)$ {\it w.r.t.} MRR &
(e) $\log(\lambda_5)$ {\it w.r.t.} MRR \\
\end{tabular}
\end{center}
\caption{Parameter analysis on the Online Boutique dataset w.r.t MRR. }
\label{fig_parameter_analysis_OB}
\vspace{-0.3cm}
\end{figure*}

\begin{figure*}
\begin{center}
\begin{tabular}{ccccc}
\hspace{-5mm}
\includegraphics[width=0.18\linewidth]{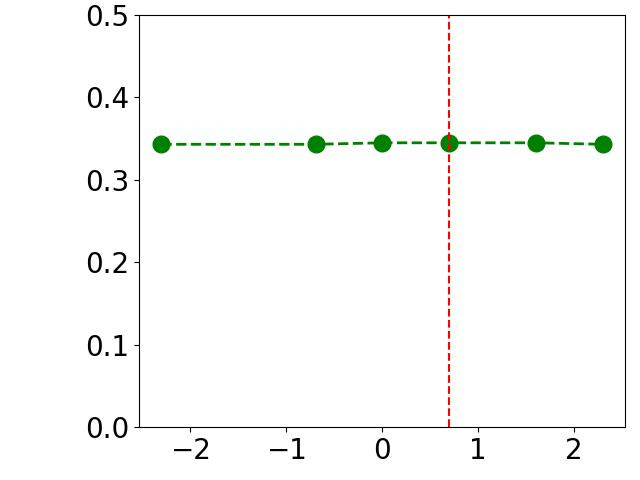} &
\includegraphics[width=0.18\linewidth]{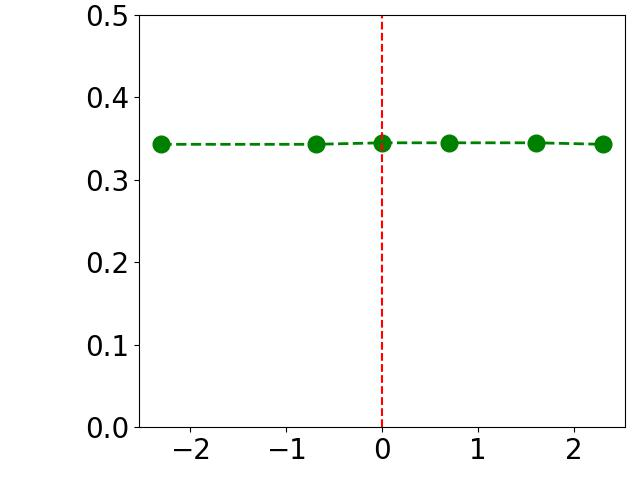} &
\includegraphics[width=0.18\linewidth]{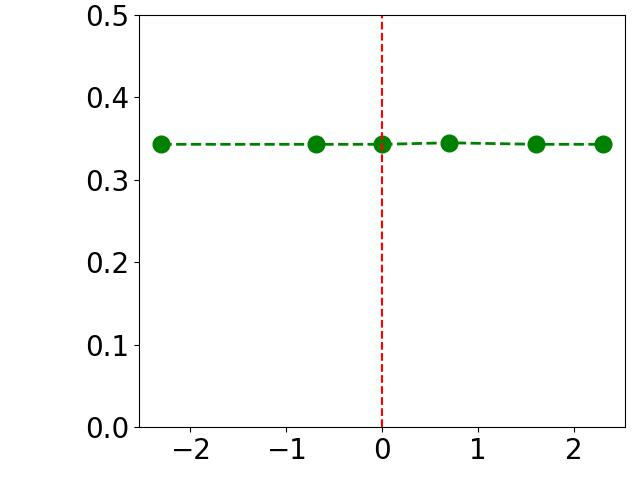} &
\includegraphics[width=0.18\linewidth]{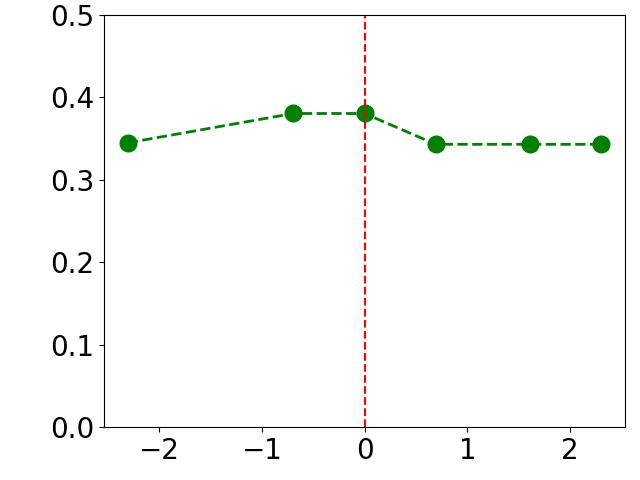} &
\includegraphics[width=0.18\linewidth]{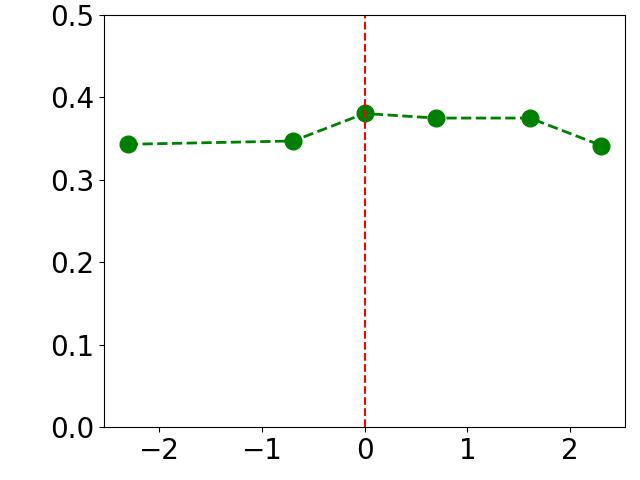}\\
(a) $\log(\lambda_1)$ {\it w.r.t.} MRR&
(b) $\log(\lambda_2)$ {\it w.r.t.} MRR &
(c) $\log(\lambda_3)$ {\it w.r.t.} MRR &
(d) $\log(\lambda_4)$ {\it w.r.t.} MRR &
(e) $\log(\lambda_5)$ {\it w.r.t.} MRR \\
\end{tabular}
\end{center}
\caption{Parameter analysis on Train Ticket dataset w.r.t MRR. }
\label{fig_parameter_analysis_TT}
\vspace{-0.3cm}
\end{figure*}

\begin{table}
\caption{Quality measurement of high-quality metric and low-quality metric on Product Review dataset. The median ranking scores are used to evaluate the quality of different metrics. The best metric is denoted as High-quality while the worst metric is denoted as Low-quality.}
\centering
\begin{tabular}{*{5}{c}}
\hline      Metric              & Case 1     &  Case 2    &   Case 3    & Case 4   \\ \hline
High-quality                    & 21         & 30         & 11          & 25 \\
Low-quality                     & 82	     & 68	      & 30	        & 40  \\
\hline
\end{tabular}
\label{table_metric_quality_measurement}
\end{table}

\subsection{How to Choose High-quality and Low-quality System Metrics?}
\label{case_stdy_median_ranking}
In the experiment, we first measure the performance of each single-modality baseline method by only using one single system metric (\textit{e.g.}, CPU usage, memory usage, rate transmit rate, \textit{etc}). Then, we select the system metric with the highest median ranking score as the high-quality system metric denoted $M^+$, and the system metric with the lowest median ranking score as the low-quality system metric denoted $M^-$. The ranking results are shown in Table~\ref{table_metric_quality_measurement}.

\subsection{Additional Parameter Analysis}
\label{Parameter_analysis_2}
In this subsection, we delve into an analysis of parameter sensitivity within the \method\ framework on the Online Boutique and Train Ticket datasets, specifically examining the impact of variations in $\lambda_1$, $\lambda_2$, $\lambda_3$, $\lambda_4$, and $\lambda_5$. Figure~\ref{fig_parameter_analysis_OB} and Figure~\ref{fig_parameter_analysis_TT} present the experimental results with respect to Mean Reciprocal Rank (MRR), where the x-axis is $\log(\lambda_i), i\in[1, 2, 3, 4, 5]$ and the y-axis is MRR. By observations on Figure~\ref{fig_parameter_analysis_OB}, we find that the value of $\lambda_1$, $\lambda_2$, $\lambda_3$, $\lambda_4$, and $\lambda_5$ does not influence the performance of \method\ on Online Boutique dataset. Our conjecture for this observation is that the number of system entities is only 10 and it's an easy task to identify the root cause by our method. Based on the experimental results on the Train Ticket dataset, we found that the change of the values for $\lambda_1$, $\lambda_2$, and $\lambda_3$ do not have a great impact on the performance of \method. \method\ achieves the best result with $\lambda_5=1$ on the Train Ticket dataset.

\begin{table}
\caption{Ablation study on three datasets evaluated by MAP@K.}
\centering
\begin{tabular}{*{4}{c}}
\hline      Model       & Product Review     &  Online Boutique      &   Train Ticket   \\ \hline
\hline      -           & MAP@10    &  MAP@5                &   MAP@10   \\ \hline
\method                 & \textbf{1.0}       & \textbf{0.96}                  & \textbf{0.386} \\
\method-V               & 0.98      & 0.92                  & 0.385 \\ 
\method-O               & 0.96      & \textbf{0.96}                  & 0.357 \\ 
\method-N               & 0.94      & 0.88                  & 0.371 \\
\method-E               & 0.96      & 0.84                  & 0.357 \\
\hline
\end{tabular}
\label{table_ablation_study_map10}
\end{table} 

\subsection{Additional Results for Case Study}
\label{ablation_study_2}
Table~\ref{table_ablation_study_map10} shows the performance evaluated by MAP@K. Comparing the performance of \method\ with other variants, removing any component of the proposed methods consistently results in performance degradation. For instance, removing the edge loss causes the performance to drop by 12\% on the Online Boutique dataset while removing the node loss leads to a 6\% performance reduction on the Product Review dataset.
